# Supplementary material for: CLIP meets DINO for Tuning Zero-Shot Classifier using Unlabeled Image Collections
Source: arXiv:2411.19346 source file (2025-04-10)
Supplement: Supplementary file 1 [file suppl_4.tex]

% FOR SUPPLEMENTARY

\begin{table}[H]
\setlength{\tabcolsep}{4pt}
    \centering % Center the table
    \caption{\textnormal{\textbf{.}}}
    \small % Adjust font size here
    \begin{tabular}{lccccccc}
    \toprule
     & \rotatebox{90}{EuroSAT} & \rotatebox{90}{Caltech101} & \rotatebox{90}{Oxford-Pets} & \rotatebox{90}{Flowers-102} & \rotatebox{90}{SUN397} & \rotatebox{90}{CIFAR100} \\
    \midrule
    # of training images  \\
    # of classes \\
    Avg. # of images per class \\
    Proportion \\
    k \\
    \bottomrule
    \end{tabular}
    \label{tab:suppl4}
\end{table}
